# Supplementary material for: Rethinking The Uniformity Metric in Self-Supervised Learning
Source: arXiv:2403.00642 source file (2024-04-26)
Supplement: Supplementary file 1 [file appendix.tex]

%%%%%%%%%%%%%%%%%%%%%%%%%%%%%%%%%%%%%%%%%%%%%%%%%%%%%%%
\section{Proof of the Claim~\ref{proof:maximum uniformity}}
\label{sec:appendix theorem}

\begin{proof}
As $\m Z \sim \mathcal{N}(\m 0, \sigma^2\m I_m)$, for any orthogonal matrix $\m U$:
\begin{align}
\hat{\m Z} = \m U \m Z &\sim \mathcal{N}(\m U\m 0, \sigma^2\m U\m I_m \m U^T),  &&  (\textrm{ by Lemma~\ref{theorem:gaussian orthogonal}}) \nonumber  \\
& ~\sim \mathcal{N}(\m 0, \sigma^2\m I_m)  &&  (\m U\m 0 = \m 0, \m U\m I_m \m U^T =\m U \m U^T =\m I_m), \nonumber
\end{align}

%Since $\m U\m 0 = \m 0$ and  $\sigma^2\m U\m I_m \m U^T =\sigma^2\m U \m U^T =\sigma^2\m I_m$, 
Since the random variable $\hat{\m Z}~\sim \mathcal{N}(\m 0, \sigma^2\m I_m)$, $\hat{\m Z}$ is identically distributed with the random variable $\m Z$. We denote \textbf{i}dentically \textbf{d}istributed operation as $\hat{\m Z} \overset{id}{\leftrightarrow} \m Z$. For the $l_2$-normalized variables:
\begin{align}
\m Y=\m Z/\Vert \m Z \Vert_2, \quad \hat{\m Y}=\hat{\m Z}/\Vert \hat{\m Z} \Vert_2, \quad \hat{\m Y} \overset{id}{\leftrightarrow} \m Y. \nonumber
\end{align}
Since $\Vert \m U \m Z \Vert_2=\sqrt{(\m U \m Z)^T(\m U \m Z)}=\sqrt{\m Z^T \m U^T \m U \m Z} = \sqrt{\m Z^T \m Z} =\Vert \m Z \Vert_2$,
\begin{align}
\hat{\m Y} = \frac{\m U \m Z}{\Vert\m U \m Z \Vert_2} =  \frac{\m U \m Z}{\Vert \m Z \Vert_2} = \m U \m Y, \nonumber
\end{align}
Therefore, $\m Y \overset{id}{\leftrightarrow} \m U \m Y$ for any orthogonal transformation $\m U$. Finally, we have Lemma~\ref{theorem:transofmr} proved.

Therefore, $\m Y$ is an identically distributed operation as $\m U \m Y$ after an arbitrary orthogonal transformation. To conclude that the random variable $\m Y$ uniformly distributes on the on the surface of the unit hypersphere $\mathcal{S}^{m-1}=\{\m y \in \mathbb{R}^m:\Vert \m y\Vert_2 = 1 \}$, here we use \textbf{the proof by contradiction}.

Let us assume the opposite of the above conclusion:  $\m Y $ does not uniformly distribute on the surface of the unit hypersphere $\mathcal{S}^{m-1}$. In other words, the density of each specified-sized area in  $\m Y $ is not identical for the unit hypersphere $\mathcal{S}^{m-1}$.
The random variable $\m Y$ has a continuous density $\rho$. 
Suppose that for $\m r_1, \m r_2 \in \mathcal{S}^{m-1}$, $\m r_1 \neq \m r_2$ and $\rho(\m r_1)>\rho(\m r_2)$, there exists a radius $\epsilon$ for any $l_2$-norm (also holds for other norms) such that on
\begin{align} \small
\nonumber & \mathcal{D}_1 = \{\m r\in \mathcal{S}^{m-1}: \Vert \m r - \m r_1 \Vert_2 < \epsilon \} ,\\\nonumber
& \mathcal{D}_2 = \{\m r\in \mathcal{S}^{m-1}: \Vert \m r - \m r_2 \Vert_2 < \epsilon \} ,\nonumber
\end{align}
we still have 
\begin{align}
\forall \m r \in \mathcal{D}_1, \forall \m s \in \mathcal{D}_2, \rho(\m r)>\rho(\m s).\nonumber
\end{align}
Therefore, $P(\mathcal{D}_1)>P(\mathcal{D}_2)$. Since $\m Y \overset{id}{\leftrightarrow} \m U \m Y$ according to Lemma~\ref{theorem:transofmr}, $\mathcal{D}_2$ can be obtained from $\mathcal{D}_1$ by a orthogonal transformation \footnote{ Let $\mW$ be a orthogonal transformation such that $\mW \vr_1 = \vr_2$.  $\mathcal{D}_2$ could be obtained by transforming every points from $\mathcal{D}_1$ using  orthogonal transformation $\mW$, namely   $\mathcal{D}_2 = \{\mW \vr: \vr \in \mathcal{D}_1 \} ,\nonumber$ }, which implies that $P(\mathcal{D}_1)=P(\mathcal{D}_2)$. 

Contradiction! Hence $\rho(\m r_1)=\rho(\m r_2)$ for $\forall \m r_1, \m r_2 \in \mathcal{S}^{m-1}$ and $\m r_1 \neq \m r_2$.
Therefore, $\m Y=\m Z/\Vert \m Z \Vert_2$ uniformly distributes on the hypersphere $\mathcal{S}^{m-1}$.
\end{proof}

\section{Proof of the Theorem~\ref{proof:y distribution}}
\label{sec:appendix proposition}
%%%%%%%%%%%%%%%%%%%%%%%%%%%%%%%%%%%%%%%%%%%%%%%%%%%%%%%%%%%%%%%%%

\begin{proof}
$\m Z=[z_1, z_2, \cdots, z_m] \sim \mathcal{N}(\m 0, \sigma^2 \m I_m)$, and its probability density function (pdf) can be written as:
\begin{align}
\nonumber \mathit{f}_{\scaleto{\m Z}{5pt}}(\m z) = \frac{1}{(2\pi)^{m/2}|\sigma^2 \m I_m|^{1/2}}\exp\{-\frac{1}{2} \m z^T (\sigma^2 \m I_m)^{-1} \m z\} = \frac{1}{(2\pi\sigma^2)^{m/2}}\exp\{-\frac{1}{2}\sum_{i=1}^{m}z_i^2/\sigma^2\}, \nonumber
\end{align}
We denote $\m Y = [y_1, y_2, \cdots, y_m]$. Then the mean of $i$-th variable $y_i$ can be written as below:
\begin{align}
\mathbb{E}[y_i] = \int_{z_1}\int_{z_2}\int_{\cdots}\int_{z_m}\frac{z_i}{\sqrt{\sum_i^m z_i^2}}\frac{1}{(2\pi\sigma^2)^{m/2}}\exp\{-\frac{1}{2}\sum_{i=1}^{m}z_i^2/\sigma^2\}d z_1 d z_2 \cdots d z_m,\nonumber
\end{align}
As $\frac{z_i}{\sqrt{\sum_i^m z_i^2}}$ is an odd function, $\mathbb{E}[y_i]=0$, and we further conclude $\bm \mu = \mathbb{E}[\m Y] = \m 0$. We also derive the covariance matrix of $\m Y$ according to its definition as below:
\begin{align}
\m \Sigma = \mathbb{E}[(\m Y-\mathbb{E}[\m Y])(\m Y-\mathbb{E}[\m Y])^T] = \begin{pmatrix}
\mathbb{E}[y_1^2] & \mathbb{E}[y_1 y_2] & \cdots & \mathbb{E}[y_1 y_m]\\
\mathbb{E}[y_2 y_1] & \mathbb{E}[y_2^2] & \cdots & \mathbb{E}[y_2 y_m]\\
\cdots & \cdots & \cdots & \cdots\\
\mathbb{E}[y_m y_1] & \mathbb{E}[y_m y_2] & \cdots & \mathbb{E}[y_m^2]
\end{pmatrix} \nonumber
\end{align}
Then $\mathbb{E}[y_i y_j]$ ($\forall i\neq j$) can be formulated as follows:
\begin{align}
\mathbb{E}[y_i y_j] = \int_{z_1}\int_{z_2}\int_{\cdots}\int_{z_m}\frac{z_i}{\sqrt{\sum_i^m z_i^2}}\frac{z_j}{\sqrt{\sum_i^m z_i^2}}\frac{1}{(2\pi\sigma^2)^{m/2}}\exp\{-\frac{1}{2}\sum_{i=1}^{m}z_i^2/\sigma^2\}d z_1 d z_2\cdots d z_m,\nonumber
\end{align}
As $\frac{z_i}{\sqrt{\sum_i^m z_i^2}}\frac{z_j}{\sqrt{\sum_i^m z_i^2}}$ is an odd function, $\mathbb{E}[y_i y_j]=0$ ($\forall i\neq j$). In terms of diagonal elements in $\m \Sigma$, we employ the symmetry to conclude $\mathbb{E}[y_1^2] = \mathbb{E}[y_2^2] = \cdots = \mathbb{E}[y_m^2]$. Based on this principle, we conclude $\mathbb{E}[y_i^2]=\frac{1}{m}$ via below equations:
\begin{align}
\mathbb{E}[\sum_i^m y_i^2] = m \mathbb{E}[y_i^2],\quad \mathbb{E}[\sum_i^m y_i^2] = \mathbb{E}[\frac{\sum_i^m z_i^2}{\sum_i^m z_i^2}] = 1, \nonumber
\end{align}
Therefore, $\m \Sigma = \frac{1}{m} \m I_m$.
\end{proof}

\section{Proof of the Desiderata}
\label{sec:appendix desiderata}
%%%%%%%%%%%%%%%%%%%%%%%%%%%%%%%%%%%%%%%%%%%%%%%%%%%%%%%%%%%%%%%%
To make theoretical comparison between our proposed uniformity metric $-\mathcal{W}_{2}$ and baseline metric $-\mathcal{L_U}$, we provide mathematical proof to verify whether these metrics satisfy designed desiderata in Section~\ref{sec:desiderata}. In terms of \textit{Property IPC} and \textit{Property ISC}, we can directly use their definition to demonstrate both two metrics satisfy the two constraints. Therefore, we focus more attention on other three constraints. Detailed proof can be seen in  Lemma~\ref{theorem:Lu ICC}, Lemma~\ref{theorem:Lu FCC}, Lemma~\ref{theorem:Lu FBC}, Lemma~\ref{theorem:Wp ICC}, Lemma~\ref{theorem:Wp FBC} and Lemma~\ref{theorem:Wp FCC}.

\begin{theorem}
Our proposed metric $-\mathcal{L_U}$ cannot satisfy the \textbf{Property~\ref{pro:icc}}, \textbf{Property~\ref{pro:fcc}}, and \textbf{Property~\ref{pro:fbc}}.
\end{theorem}

\begin{theorem}
The baseline metric $-\mathcal{W}_{2}$ could well satisfy the \textbf{Property~\ref{pro:icc}}, \textbf{Property~\ref{pro:fcc}}, and \textbf{Property~\ref{pro:fbc}}.
\end{theorem}

\begin{lemma}
\label{theorem:Lu ICC}
Suppose a set of random variables $\mathcal{D} = \{\m z_1, \m z_2, ..., \m z_n\}$ ($\m z_i \in \mathbb{R}^m$), and a function as follows:
\begin{align}
\mathcal{L_U}({\mathcal{D}}) \triangleq \log \frac{1}{n(n-1)/2} \sum_{i=2}^{n} \sum_{j=1}^{i-1} e^{-t \Vert \frac{\m z_i}{\Vert \m z_i \Vert} - \frac{\m z_j}{\Vert \m z_j \Vert}\Vert_2^{2}}, \nonumber
\end{align}
Then $\mathcal{L_U}(\mathcal{D} \cup \mathcal{D}) \geq \mathcal{L_U}(\mathcal{D})$. $\mathcal{L_U}(\mathcal{D} \cup \mathcal{D}) = \mathcal{L_U}(\mathcal{D})$ if and only if $\m z_1 = \m z_2 = ... = \m z_n$.
\end{lemma}
\begin{proof}
\begin{align}
\mathcal{L_U}(\mathcal{D} \cup \mathcal{D}) & \triangleq \log \frac{1}{2n(2n-1)/2} (4 \sum_{i=2}^{n} \sum_{j=1}^{i-1} e^{-t \Vert \frac{\m z_i}{\Vert \m z_i \Vert} - \frac{\m z_j}{\Vert \m z_j \Vert}\Vert_2^{2}} + \sum_{i=1}^{n} e^{-t \Vert \frac{\m z_i}{\Vert \m z_i \Vert} - \frac{\m z_i}{\Vert \m z_i \Vert}\Vert_2^{2}}) \nonumber\\
& = \log \frac{1}{2n(2n-1)/2} (4\sum_{i=2}^{n} \sum_{j=1}^{i-1} e^{-t \Vert \frac{\m z_i}{\Vert \m z_i \Vert} - \frac{\m z_j}{\Vert \m z_j \Vert}\Vert_2^{2}} + n), \nonumber\\ \nonumber
\end{align}
We set $G = \sum_{i=2}^{n} \sum_{j=1}^{i-1} e^{-t \Vert \frac{\m z_i}{\Vert \m z_i \Vert} - \frac{\m z_j}{\Vert \m z_j \Vert}\Vert_2^{2}}$, and then we have:
\begin{align}
G =  \sum_{i=2}^{n} \sum_{j=1}^{i-1} e^{-t \Vert \frac{\m z_i}{\Vert \m z_i \Vert} - \frac{\m z_j}{\Vert \m z_j \Vert}\Vert_2^{2}} \leq  \sum_{i=2}^{n} \sum_{j=1}^{i-1} e^{-t \Vert \frac{\m z_i}{\Vert \m z_i \Vert} - \frac{\m z_i}{\Vert \m z_i \Vert}\Vert_2^{2}} = n(n-1)/2 \nonumber
\end{align}
$G = n(n-1)/2$ if and only if $\m z_1 = \m z_2 = ... = \m z_n$.
\begin{align}
\mathcal{L_U}(\mathcal{D} \cup \mathcal{D}) - \mathcal{L_U}({\mathcal{D}})  & = \log \frac{4G + n}{2n(2n-1)/2} - \log \frac{G}{n(n-1)/2} \nonumber\\
& = \log \frac{(4G + n )n(n-1)/2}{2nG(2n-1)/2} 
= \log \frac{(4G + n)(n-1)}{4nG-2G} \nonumber\\
& = \log \frac{4nG-4G+ n^2-n}{4nG -2G} \geq \log 1 = 0. \nonumber
\end{align}
$\mathcal{L_U}(\mathcal{D} \cup \mathcal{D}) = \mathcal{L_U}(\mathcal{D})$ if and only if $G = n(n-1)/2$, which requires $\m z_1 = \m z_2 = ... = \m z_n$.
\end{proof}

\begin{lemma}
\label{theorem:Lu FCC}
Suppose a set of random variables $\mathcal{D} = \{\m z_1, \m z_2, ..., \m z_n\}$ ($\m z_i \in \mathbb{R}^m$), and a function as follows:
\begin{align}
\mathcal{L_U}({\mathcal{D}}) \triangleq \log \frac{1}{n(n-1)/2} \sum_{i=2}^{n} \sum_{j=1}^{i-1} e^{-t\Vert \frac{\m z_i}{\Vert \m z_i \Vert} - \frac{\m z_j}{\Vert \m z_j \Vert}\Vert_2^{2}}, \nonumber
\end{align}
Then $\mathcal{L_U}(\mathcal{D} \oplus \mathcal{D}) = \mathcal{L_U}(\mathcal{D})$. 
\end{lemma}
\begin{proof}
Given $\m z_i = [z_{i1}, z_{i2}, ..., z_{im}]^{T}$, and $\m z_j = [z_{j1}, z_{j2}, ..., z_{jm}]^{T}$, and we set $\hat{\m z}_i = \m z_i \oplus \m z_i$ and $\hat{\m z}_j = \m z_j \oplus \m z_j$, Then:
\begin{align}
\mathcal{L_U}(\mathcal{D} \oplus \mathcal{D}) \triangleq \log \frac{1}{n(n-1)/2} \sum_{i=2}^{n} \sum_{j=1}^{i-1} e^{-t\Vert \frac{\hat{\m z}_i}{\Vert \hat{\m z}_i \Vert} - \frac{\hat{\m z}_j}{\Vert \hat{\m z}_j \Vert}\Vert_2^{2}}, \nonumber
\end{align}
As $\hat{\m z}_i = [z_{i1}, z_{i2}, ..., z_{im}, z_{i1}, z_{i2}, ..., z_{im}]^{T}$ and $\hat{\m z}_j = [z_{j1}, z_{j2}, ..., z_{jm}, z_{j1}, z_{j2}, ..., z_{jm}]^{T}$, then $\Vert \hat{\m z}_i \Vert = \sqrt{2}\Vert \m z_i \Vert$, $\Vert \hat{\m z}_j \Vert = \sqrt{2}\Vert \m z_j \Vert$, and $\langle \hat{\m z}_i, \hat{\m z}_j \rangle=2\langle \m z_i, \m z_j \rangle$, therefore: 
\begin{align}
\Vert \frac{\hat{\m z}_i}{\Vert \hat{\m z}_i \Vert} - \frac{\hat{\m z}_j}{\Vert \hat{\m z}_j \Vert}\Vert_2^{2} = 2 - 2\frac{\langle \hat{\m z}_i, \hat{\m z}_j \rangle}{\Vert \hat{\m z}_i \Vert\Vert \hat{\m z}_j \Vert} =  2 - 2\frac{2\langle \m z_i, \m z_j \rangle}{\sqrt{2}\Vert \m z_i \Vert \sqrt{2} \Vert \m z_j \Vert} = \Vert \frac{\m z_i}{\Vert \m z_i \Vert} - \frac{\m z_j}{\Vert \m z_j \Vert}\Vert_2^{2}, \nonumber
\end{align}
Therefore, $\mathcal{L_U}(\mathcal{D} \oplus \mathcal{D}) = \mathcal{L_U}(\mathcal{D})$.
\end{proof}

\begin{lemma}
\label{theorem:Lu FBC}
Suppose a set of random variables $\mathcal{D} = \{\m z_1, \m z_2, ..., \m z_n\}$ ($\m z_i \in \mathbb{R}^m$), and a function as follows:
\begin{align}
\mathcal{L_U}({\mathcal{D}}) \triangleq \log \frac{1}{n(n-1)/2} \sum_{i=2}^{n} \sum_{j=1}^{i-1} e^{-t\Vert \frac{\m z_i}{\Vert \m z_i \Vert} - \frac{\m z_j}{\Vert \m z_j \Vert}\Vert_2^{2}}, \nonumber
\end{align}
Then $\mathcal{L_U}(\mathcal{D} \oplus \m 0^{k}) = \mathcal{L_U}(\mathcal{D})$. 
\end{lemma}
\begin{proof}
Given $\m z_i = [z_{i1}, z_{i2}, ..., z_{im}]^{T}$, and $\m z_j = [z_{j1}, z_{j2}, ..., z_{jm}]^{T}$, and we set $\hat{\m z}_i = \m z_i \oplus \m 0^{k}$ and $\hat{\m z}_j = \m z_j \oplus \m 0^{k}$, Then:
\begin{align}
\mathcal{L_U}(\mathcal{D} \oplus \m 0^{k}) \triangleq \log \frac{1}{n(n-1)/2} \sum_{i=2}^{n} \sum_{j=1}^{i-1} e^{-t\Vert \frac{\hat{\m z}_i}{\Vert \hat{\m z}_i \Vert} - \frac{\hat{\m z}_j}{\Vert \hat{\m z}_j \Vert}\Vert_2^{2}}, \nonumber
\end{align}
As $\hat{\m z}_i = [z_{i1}, z_{i2}, ..., z_{im}, 0, 0, ..., 0]^{T}$, and $\hat{\m z}_j = [z_{j1}, z_{j2}, ..., z_{jm}, 0, 0, ..., 0]^{T}$, then $\Vert \hat{\m z}_i \Vert = \Vert \m z_i \Vert$, $\Vert \hat{\m z}_j \Vert = \Vert \m z_j \Vert$, and $\langle \hat{\m z}_i, \hat{\m z}_j \rangle=\langle \m z_i, \m z_j \rangle$, therefore:
\begin{align}
\Vert \frac{\hat{\m z}_i}{\Vert \hat{\m z}_i \Vert} - \frac{\hat{\m z}_j}{\Vert \hat{\m z}_j \Vert}\Vert_2^{2} = 2 - 2\frac{\langle \hat{\m z}_i, \hat{\m z}_j \rangle}{\Vert \hat{\m z}_i \Vert \Vert \hat{\m z}_j \Vert} =  2 - 2 \frac{\langle \m z_i, \m z_j \rangle}{\Vert \m z_i \Vert \Vert \m z_j \Vert} = \Vert \frac{\m z_i}{\Vert \m z_i \Vert} - \frac{\m z_j}{\Vert \m z_j \Vert}\Vert_2^{2}, \nonumber
\end{align}
Therefore, $\mathcal{L_U}(\mathcal{D} \oplus \m 0^{k}) = \mathcal{L_U}(\mathcal{D})$.
\end{proof}

\begin{lemma}
\label{theorem:Wp ICC}
Suppose a set of random variables $\mathcal{D} = \{\m z_1, \m z_2, ..., \m z_n\}$ ($\m z_i \in \mathbb{R}^m$), and corresponding mean vector and covariance matrix are as follows:
\begin{align}
\bm \mu = \frac{1}{n}\sum_{i=1}^{n} \m z_i/\Vert \m z_i \Vert, \quad \m \Sigma = \frac{1}{n}\sum_{i=1}^{n}(\m z_i/\Vert \m z_i \Vert - \bm \mu)^T(\m z_i/\Vert \m z_i \Vert -\bm \mu), \nonumber
\end{align}
For a function as follows:
\begin{align}
\mathcal{W}_{2} \triangleq \sqrt{\Vert \bm \mu \Vert^2_{2} + 1 + Tr(\m \Sigma) -\frac{2}{\sqrt{m}} Tr(\m \Sigma^{1/2})}, \nonumber
\end{align}
Then $\mathcal{W}_{2}(\mathcal{D} \cup \mathcal{D}) = \mathcal{W}_{2}(\mathcal{D})$.
\end{lemma}
\begin{proof}
As $\mathcal{D} \cup \mathcal{D} =  \{\m z_1, \m z_2, ..., \m z_n, \m z_1, \m z_2, ..., \m z_n\}$, then its mean vector and covariance matrix can be formulated as follows:
\begin{align}
\hat{\bm \mu} = \frac{1}{2n}\sum_{i=1}^{n} 2 \m z_i/\Vert \m z_i \Vert = \bm \mu, \quad \hat{\m \Sigma} = \frac{1}{2n}\sum_{i=1}^{n}2(\m z_i/\Vert \m z_i \Vert - \hat{\bm \mu})^T(\m z_i/\Vert \m z_i \Vert -\hat{\bm \mu}) = \m \Sigma, \nonumber
\end{align}
Therefore:
\begin{align}
\mathcal{W}_{2}(\mathcal{D} \cup \mathcal{D}) \triangleq \sqrt{\Vert \hat{\bm \mu}\Vert^2_{2} + 1 + Tr(\hat{\m \Sigma}) -\frac{2}{\sqrt{m}} Tr(\hat{\m \Sigma}^{1/2}}) = \mathcal{W}_{2}(\mathcal{D}). \nonumber
\end{align}
\end{proof}

\begin{lemma}
\label{theorem:Wp FBC}
Suppose a set of random variables $\mathcal{D} = \{\m z_1, \m z_2, ..., \m z_n\}$ ($\m z_i \in \mathbb{R}^m$), and corresponding mean vector and covariance matrix are as follows:
\begin{align}
\bm \mu = \frac{1}{n}\sum_{i=1}^{n} \m z_i/\Vert \m z_i \Vert, \quad \m \Sigma = \frac{1}{n}\sum_{i=1}^{n}(\m z_i/\Vert \m z_i \Vert - \bm \mu)^T(\m z_i/\Vert \m z_i \Vert -\bm \mu), \nonumber
\end{align}
For a function as follows:
\begin{align}
\mathcal{W}_{2} \triangleq \sqrt{\Vert \bm \mu \Vert^2_{2} + 1 + Tr(\m \Sigma) -\frac{2}{\sqrt{m}} Tr(\m \Sigma^{1/2})}, \nonumber
\end{align}
Then $\mathcal{W}_{2}(\mathcal{D} \oplus \m 0^{k}) > \mathcal{W}_{2}(\mathcal{D})$.
\end{lemma}
\begin{proof}
Given $\m z_i = [z_{i1}, z_{i2}, ..., z_{im}]^{T}$, and $\hat{\m z}_i = \m z_i \oplus \m 0^{k} = [z_{i1}, z_{i2}, ..., z_{im}, 0, 0, ..., 0]^{T} \in \mathbb{R}^{m+k}$, for the set: $\mathcal{D} \oplus \m 0^{k}$, its mean vector and covariance matrix can be formulated as follows:
\begin{align}
\hat{\bm \mu} = \begin{pmatrix}
\bm \mu \\
\m 0^{k}
\end{pmatrix}, \quad
\hat{\m \Sigma} = \begin{pmatrix}
\m \Sigma & \m 0^{m \times k} \\
\m 0^{k \times m} & \m 0^{k \times k}
\end{pmatrix} \nonumber
\end{align}
Therefore, $Tr(\hat{\m \Sigma}) = Tr(\m \Sigma)$, and $Tr(\hat{\m \Sigma}^{1/2}) = Tr(\m \Sigma^{1/2})$:
\begin{align}
\mathcal{W}_{2}(\mathcal{D} \oplus \m 0^{k}) & \triangleq \sqrt{\Vert \hat{\bm \mu}\Vert^2_{2} + 1 + Tr(\hat{\m \Sigma}) -\frac{2}{\sqrt{m+k}}Tr(\hat{\m \Sigma}^{1/2})} \nonumber \\
& = \sqrt{\Vert \bm \mu \Vert^2_{2} + 1 + Tr(\m \Sigma) -\frac{2}{\sqrt{m+k}} Tr(\m \Sigma^{1/2})} \nonumber \\
& > \sqrt{\Vert \bm \mu \Vert^2_{2} + 1 + Tr(\m \Sigma) -\frac{2}{\sqrt{m}} Tr(\m \Sigma^{1/2})} = \mathcal{W}_{2}(\mathcal{D}) \nonumber
\end{align}
Therefore,  $\mathcal{W}_{2}(\mathcal{D} \oplus \m 0^{k}) > \mathcal{W}_{2}(\mathcal{D})$.
\end{proof}

\begin{lemma}
\label{theorem:Wp FCC}
Suppose a set of random variables $\mathcal{D} = \{\m z_1, \m z_2, ..., \m z_n\}$ ($\m z_i \in \mathbb{R}^m$), and corresponding mean vector and covariance matrix are as follows:
\begin{align}
\bm \mu = \frac{1}{n}\sum_{i=1}^{n} \m z_i/\Vert \m z_i \Vert, \quad \m \Sigma = \frac{1}{n}\sum_{i=1}^{n}(\m z_i/\Vert \m z_i \Vert - \bm \mu)^T(\m z_i/\Vert \m z_i \Vert -\bm \mu), \nonumber
\end{align}
For a function as follows:
\begin{align}
\mathcal{W}_{2} \triangleq \sqrt{\Vert \bm \mu \Vert^2_{2} + 1 + Tr(\m \Sigma) -\frac{2}{\sqrt{m}} Tr(\m \Sigma^{1/2})}, \nonumber
\end{align}
Then $\mathcal{W}_{2}(\mathcal{D} \oplus \mathcal{D}) > \mathcal{W}_{2}(\mathcal{D})$.
\end{lemma}
\begin{proof}
Given $\m z_i = [z_{i1}, z_{i2}, ..., z_{im}]^{T}$, and $\hat{\m z}_i = \m z_i \oplus \m z_i=[z_{i1}, z_{i2}, ..., z_{im}, z_{i1}, z_{i2}, ..., z_{im}]^{T} \in \mathbb{R}^{2m}$, for the set: $\mathcal{D} \oplus \mathcal{D}$, its mean vector and covariance matrix can be formulated as follows:
\begin{align}
\hat{\bm \mu} = \begin{pmatrix}
\bm \mu/\sqrt{2} \\
\bm \mu/\sqrt{2}
\end{pmatrix}, \quad
\hat{\m \Sigma} = \begin{pmatrix}
\m \Sigma/2 & \m \Sigma/2 \\
\m \Sigma/2 & \m \Sigma/2
\end{pmatrix} \nonumber
\end{align}
As $\hat{\m \Sigma}^{1/2}=\begin{pmatrix}
\m \Sigma^{1/2}/2 & \m \Sigma^{1/2}/2 \\
\m \Sigma^{1/2}/2 & \m \Sigma^{1/2}/2
\end{pmatrix}$, $Tr(\hat{\m \Sigma}) = Tr(\m \Sigma)$ and $Tr(\hat{\m \Sigma}^{1/2})=Tr(\m \Sigma^{1/2})$,
Therefore, 
\begin{align}
\mathcal{W}_{2}(\mathcal{D} \oplus \mathcal{D}) & \triangleq \sqrt{\Vert \hat{\bm \mu}\Vert^2_{2} + 1 + Tr(\hat{\m \Sigma}) -\frac{2}{\sqrt{2m}}Tr(\hat{\m \Sigma}^{1/2})} \nonumber \\
& = \sqrt{\Vert \bm \mu \Vert^2_{2} + 1 + Tr(\m \Sigma) -\frac{2}{\sqrt{2m}} Tr(\m \Sigma^{1/2})}, \nonumber \\
& > \sqrt{\Vert \bm \mu \Vert^2_{2} + 1 + Tr(\m \Sigma) -\frac{2}{\sqrt{m}} Tr(\m \Sigma^{1/2})} = \mathcal{W}_{2}(\mathcal{D}), \nonumber
\end{align}
Therefore, $\mathcal{W}_{2}(\mathcal{D} \oplus \mathcal{D}) > \mathcal{W}_{2}(\mathcal{D})$.
\end{proof}
%%%%%%%%%%%%%%%%%%%%%%%%%%%%%%%%%%%%%%%%%%%%%%%%%%%%%%%%%%%%%%%%%
\section{Distribution Distances over Gaussian Distribution}
\label{sec:other distribution distance}
In this section, besides Wasserstein distance over Gaussian distribution, as shown in Theorem~\ref{theorem:Wasserstein Distance}, we also discuss using other distribution distances as \emph{uniformity} metrics, and make comparisons with Wasserstein distance. As provided Kullback-Leibler Divergence and  Bhattacharyya Distance over Gaussian distribution in Theorem~\ref{theorem:kl distance} and in Theorem~\ref{theorem:bd distance}, both calculations require the covariance matrix is a full rank matrix, making them hard to be used to conduct dimensional collapse analysis. On the contrary, our proposed \emph{uniformity} metric via Wasserstein distance is free from such requirement on the covariance matrix, making it easier to be widely used in practical scenarios.
\begin{theorem}
\label{theorem:Wasserstein Distance}
\textbf{Wasserstein Distance}~(\cite{Olkin1982TheDB}) Suppose two random variables $\m Z_1 \sim \mathcal{N}(\bm \mu_1, \m \Sigma_1)$ and $\m Z_2 \sim \mathcal{N}(\bm \mu_2, \m \Sigma_2)$ obey multivariate normal distributions, then $l_2$-Wasserstein distance between $\m Z_1$ and $\m Z_2$ is:
\begin{align}
\mathcal{W}_2(\m Z_1, \m Z_2) = \sqrt{\Vert \bm \mu_1 - \bm \mu_2\Vert^2_{2} + Tr(\m \Sigma_1 + \m \Sigma_2 -2(\m \Sigma_2^{1/2}\m \Sigma_1 \m \Sigma_2^{1/2})^{1/2})},
\label{eq:wasserstein distance definition}
\end{align}
\end{theorem}
\begin{theorem}
\label{theorem:kl distance}
\textbf{Kullback-Leibler Divergence}~(\cite{Lindley1959InformationTA}) Suppose two random variables $\m Z_1 \sim \mathcal{N}(\bm \mu_1, \m \Sigma_1)$ and $\m Z_2 \sim \mathcal{N}(\bm \mu_2, \m \Sigma_2)$ obey multivariate normal distributions, then Kullback-Leibler divergence between $\m Z1$ and $\m Z_2$ is:
\begin{align}
\mathcal{D}_{KL}(\m Z_1, \m Z_2) = \frac{1}{2}((\bm \mu_1-\bm \mu_2)^T \m \Sigma_2^{-1}(\bm \mu_1-\bm \mu_2) + Tr(\m \Sigma_2^{-1}\m \Sigma_1-\m I) + \ln{\frac{\det{\m \Sigma_2}}{\det \m \Sigma_1}}), \nonumber
\label{eq:kl distance}
\end{align}
\end{theorem}

\begin{theorem}
\label{theorem:bd distance}
\textbf{Bhattacharyya Distance}~(\cite{Bhattacharyya1943OnAM}) Suppose two random variables $\m Z_1 \sim \mathcal{N}(\bm \mu_1, \m \Sigma_1)$ and $\m Z_2 \sim \mathcal{N}(\bm \mu_2, \m \Sigma_2)$ obey multivariate normal distributions, $\m \Sigma = \frac{1}{2}(\m \Sigma_1 + \m \Sigma_2)$, then bhattacharyya distance between $\m Z1$ and $\m Z_2$ is:
\begin{align}
\mathcal{D}_{B}(\m Z_1, \m Z_2) = \frac{1}{8}(\bm \mu_1-\bm \mu_2)^T \m \Sigma^{-1}(\bm \mu_1-\bm \mu_2) + \frac{1}{2}\ln \frac{\det \m \Sigma}{\sqrt{\det \m \Sigma_1 \det \m \Sigma_2}}, \nonumber
\end{align}
\end{theorem}

%%%%%%%%%%%%%%%%%%%%%%%%%%%%%%%%%%%%%%%%%%%%%%%%%%%%%%%%%%%%%%%%%%%%%%%%%%%%%
\section{The definition of Wasserstein Distance}
\label{sec:definition of wasserstein distance}
\begin{definition}
\textbf{Wasserstein Distance or \emph{Earth-Mover} Distance} with $p$ norm is defined as below:
\begin{equation}
W_{p}(\mathbb{P}_r, \mathbb{P}_g) = (\inf_{\gamma \in \Pi(\mathbb{P}_r ,\mathbb{P}_g)} \mathbb{E}_{(x, y) \sim \gamma}\big[\|x - y\|^{p}\big])^{1/p}~,
\label{eq:def wasserstein distance}
\end{equation}
where $\Pi(\mathbb{P}_r,\mathbb{P}_g)$ denotes the set of all joint distributions $\gamma(x,y)$ whose marginals are respectively $\mathbb{P}_r$ and $\mathbb{P}_g$. Intuitively, when viewing each distribution as a unit amount of earth/soil, Wasserstein Distance or \emph{Earth-Mover} Distance takes the minimum cost of transporting ``mass'' from $x$ to $y$ in order to transform the distribution
$\mathbb{P}_r$ into the distribution $\mathbb{P}_g$.
\end{definition}
As visualized in Fig.~\ref{fig:curved density}, we use 50000 samples to calculate the binning density for $y_i$ and $\hat{y}_i$ ($m=2^9$ and the number of bins is 101). To measure the distribution distance between $y_i$ and $\hat{y}_i$, we first instantiate $\mathbb{P}_r$ and $\mathbb{P}_g$ with the binning density of $y_i$ and $\hat{y}_i$, respectively. Then we use $W_{1}(\mathbb{P}_r, \mathbb{P}_g)$ as the distribution distance, as visualized in Fig.~\ref{fig:earth mover distance}. In terms of the samples used in the calculation of binning density, we sample them from $y_i$ and $\hat{y}_i$ ten times with different seeds.

%%%%%%%%%%%%%%%%%%%%%%%%%%%%%%%%%%%%%%%%%%%%%%%%%%%%%%
\section{Empirical Analysis on the Dimensional Collapse}
\label{sec:empirical analysis on dimensional collapse}
In this section, we use synthetic data with various specified degrees of dimensional collapse, to check whether the two metrics ($\mathcal{L_U}$ and $\mathcal{W}_{2}$) are capable to identify dimensional collapse. As shown in Fig.~\ref{fig:lu collapse level} and Fig.~\ref{fig:Wp collapse level}, $\mathcal{W}_{2}$ has the good ability to capture salient sensitivity to collapse level, while $\mathcal{L_U}$ fails. We also find  $\mathcal{L_U}$ becomes indistinguishable with different degrees of dimension collapse ($\eta = 25\%, 50\%, \textrm{and} 75\%$) when the dimension $m$ becomes large (e.g., $m \geq 2^8$), as visualized in Fig.~\ref{fig:dimension lu}. On the contrary, our proposed $\mathcal{W}_{2}$ is constant to the dimension number under a specific  degree of dimension collapse; $\mathcal{W}_{2}$ only depends on the degree of dimension collapse and is independent of the dimension number, as shown in Fig.~\ref{fig:dimension wp}.
\begin{figure*}[h]
    \small
	\centering
	\subfigure[Collapse analysis via $\mathcal{L_U}$]{ 
		\label{fig:lu collapse level}  
		\includegraphics[width=0.43\textwidth]{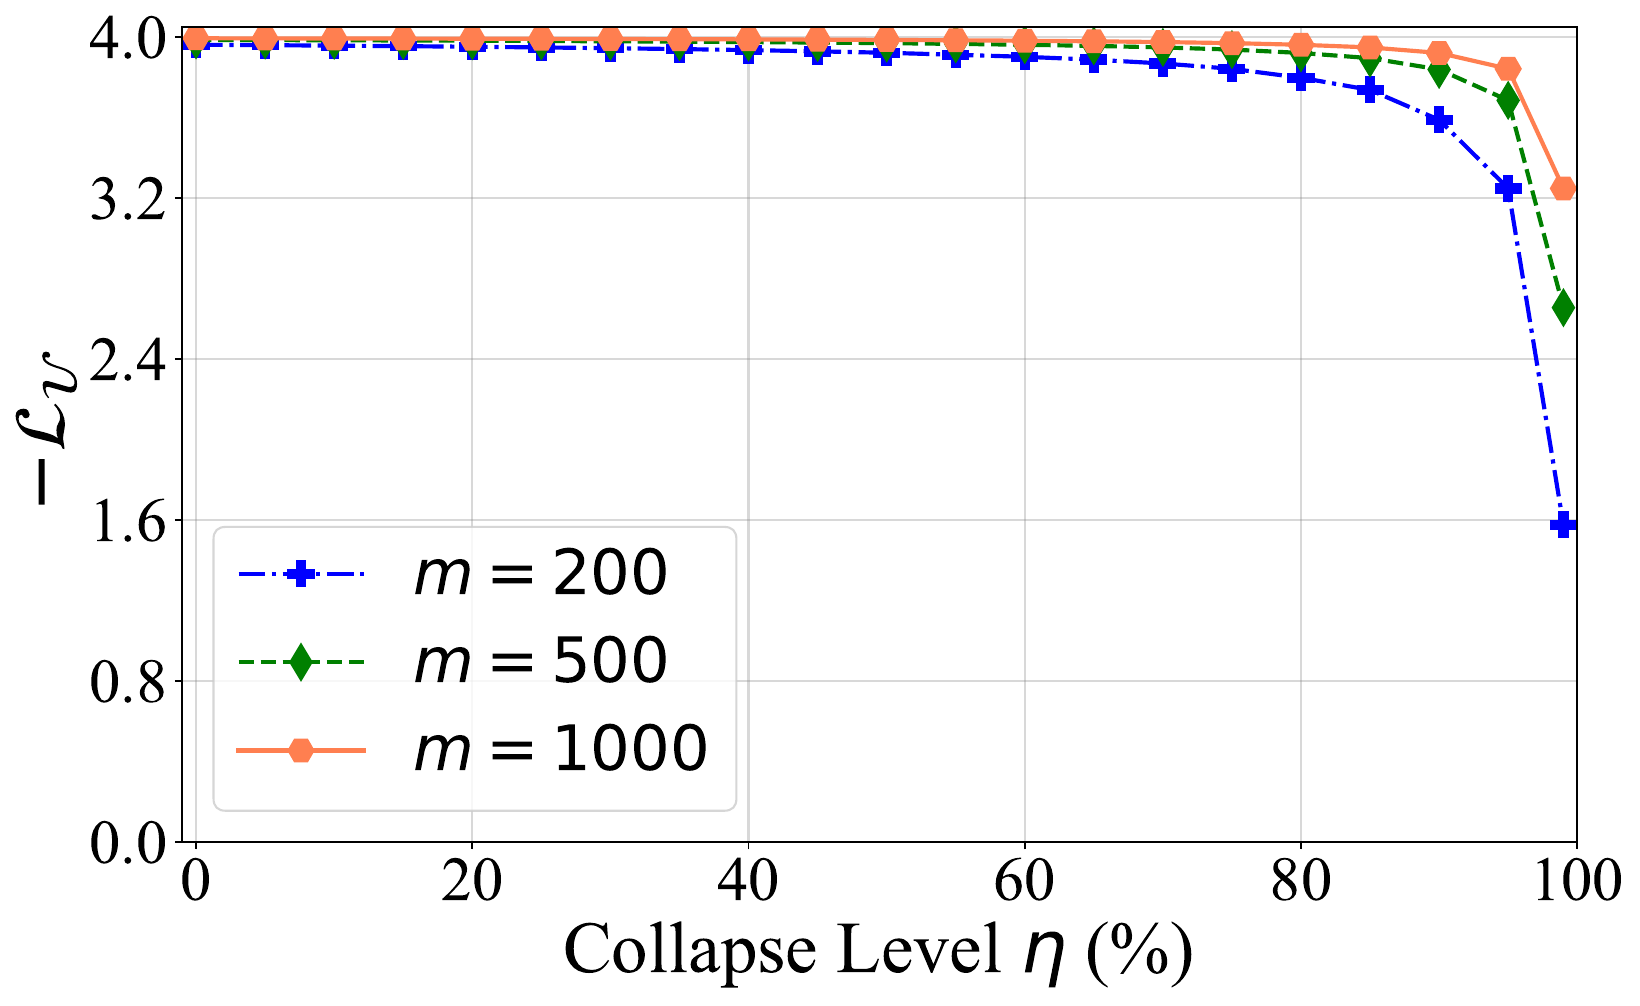}
	}
	\hspace{-0.2cm}
	\subfigure[Collapse analysis via $\mathcal{W}_{2}$]{
		\label{fig:Wp collapse level}
		\includegraphics[width=0.43\textwidth]{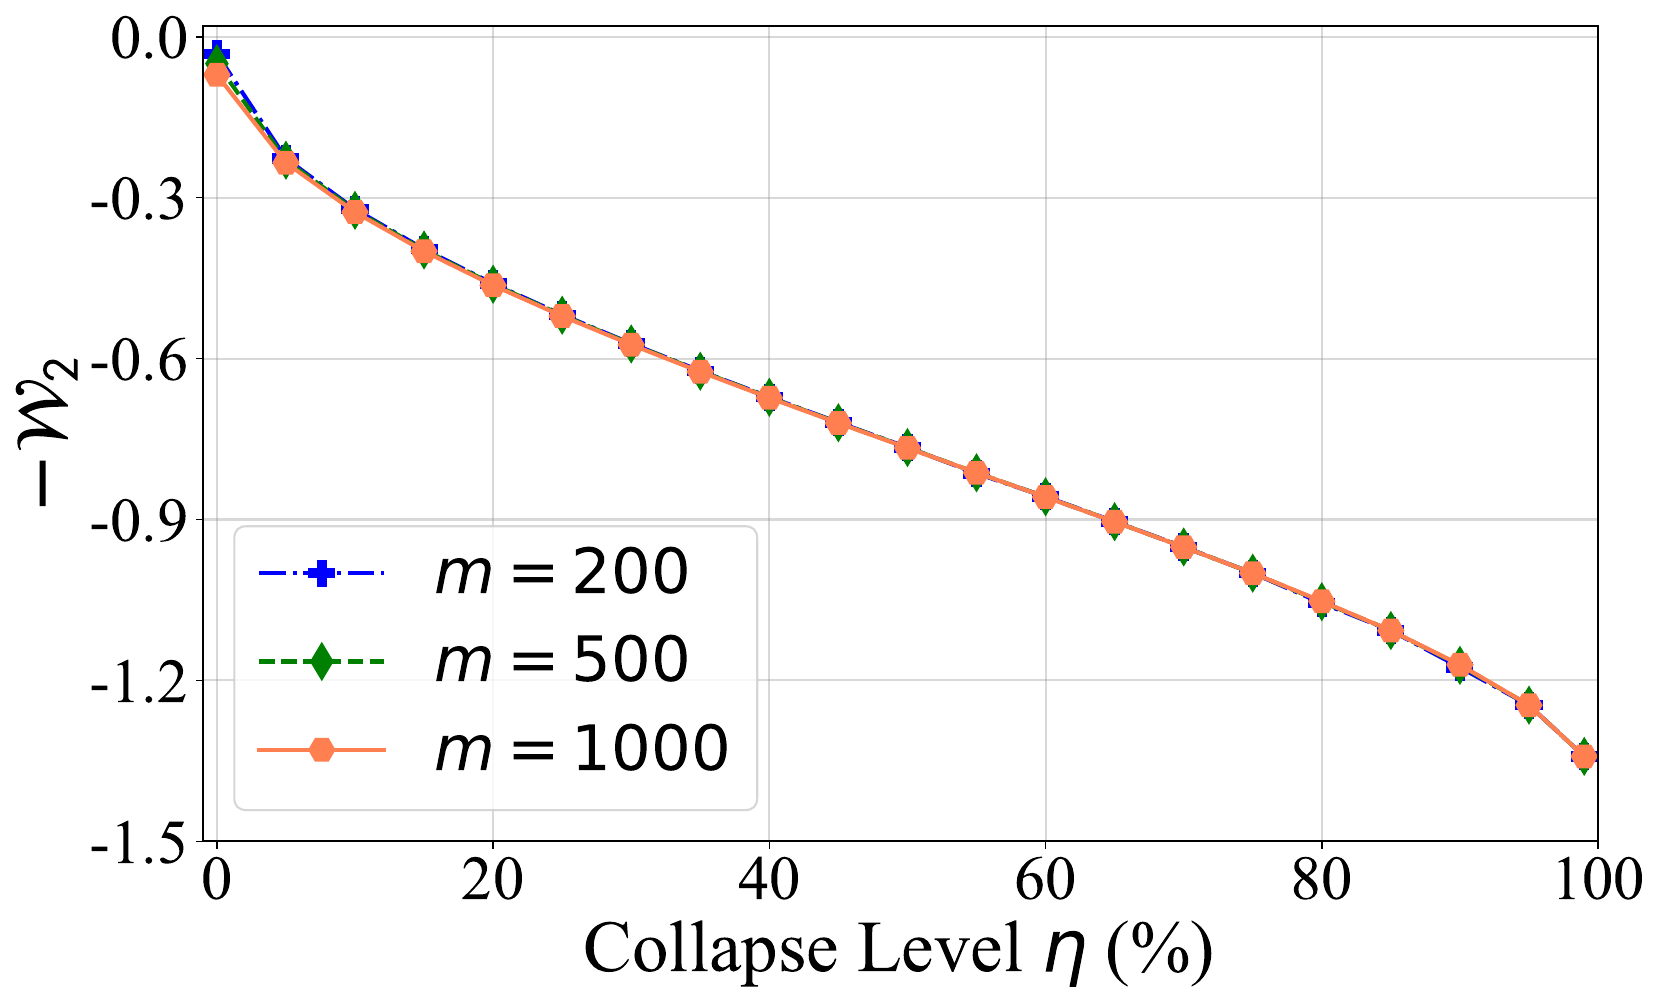}
	}
	\caption{\small{Empirical analysis on different degrees of dimension collapse. $\mathcal{W}_{2}$ well captures salient sensitivity to collapse level, while $\mathcal{L_U}$ fails.}}
	\vspace{-4mm}
	\label{fig:collapse analysis on various collapse level}
\end{figure*}

\begin{figure*}[h]
    \small
	\centering
	\subfigure[Collapse analysis via $\mathcal{L_U}$] { 
		\label{fig:dimension lu}
		\includegraphics[width=0.43\textwidth]{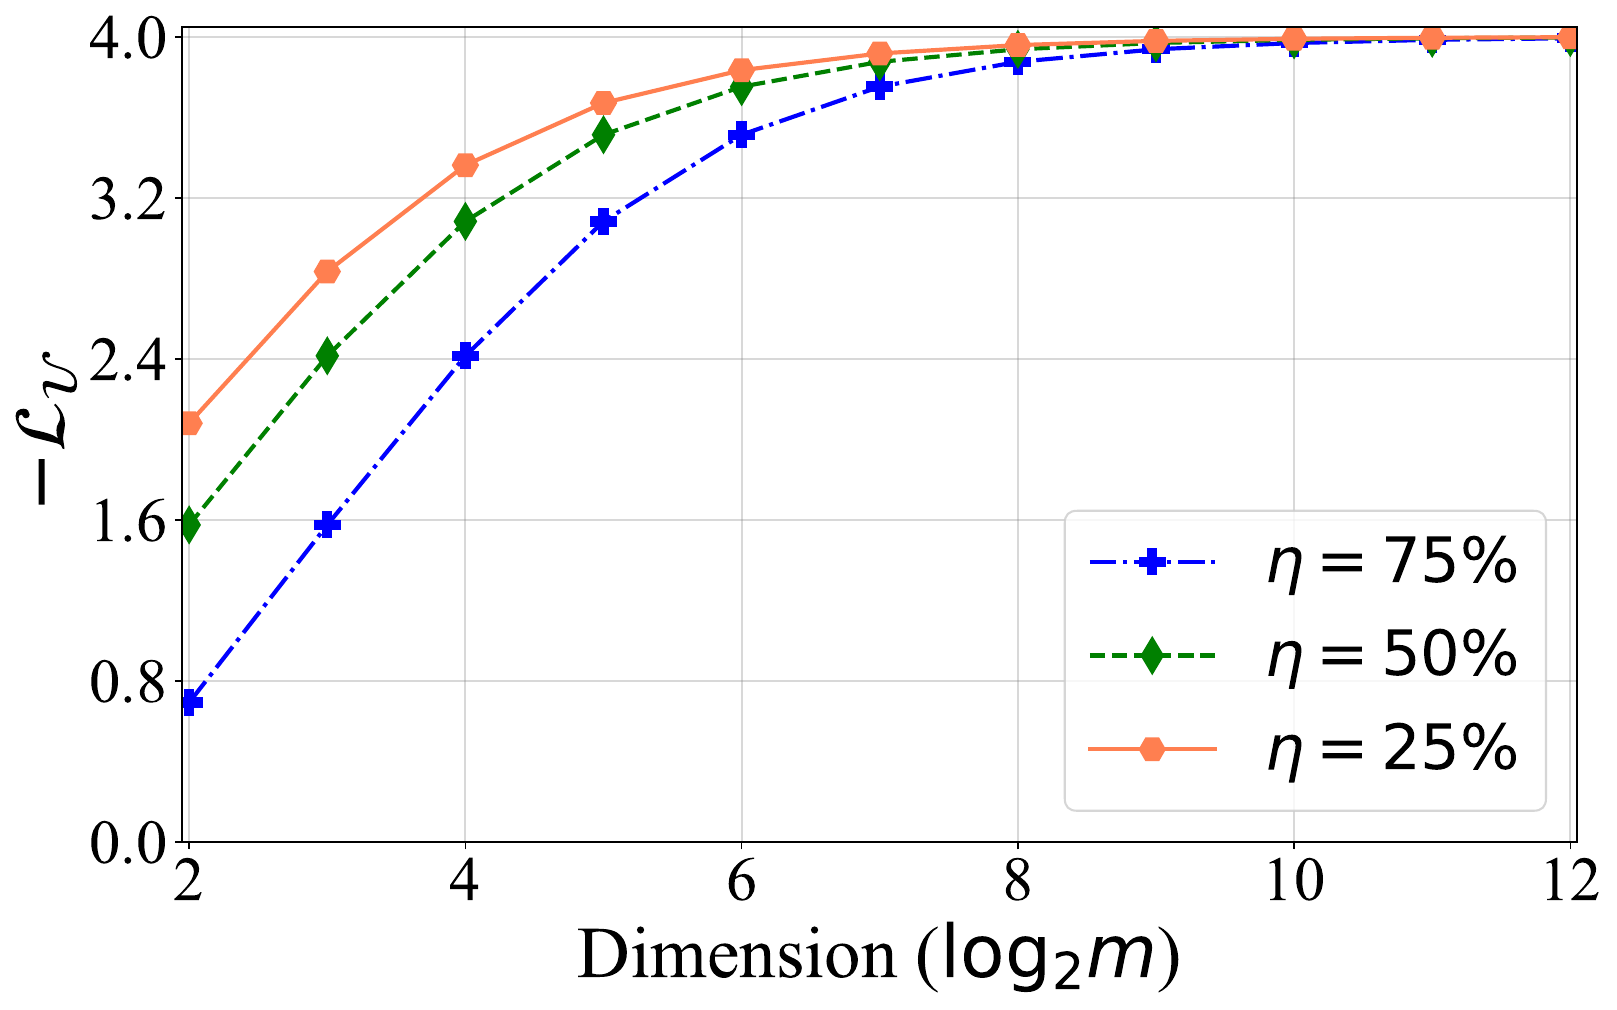}     
	}
	\hspace{-0.2cm}
	\subfigure[Collapse analysis via $\mathcal{W}_{2}$]{
		\label{fig:dimension wp}
		\includegraphics[width=0.43\textwidth]{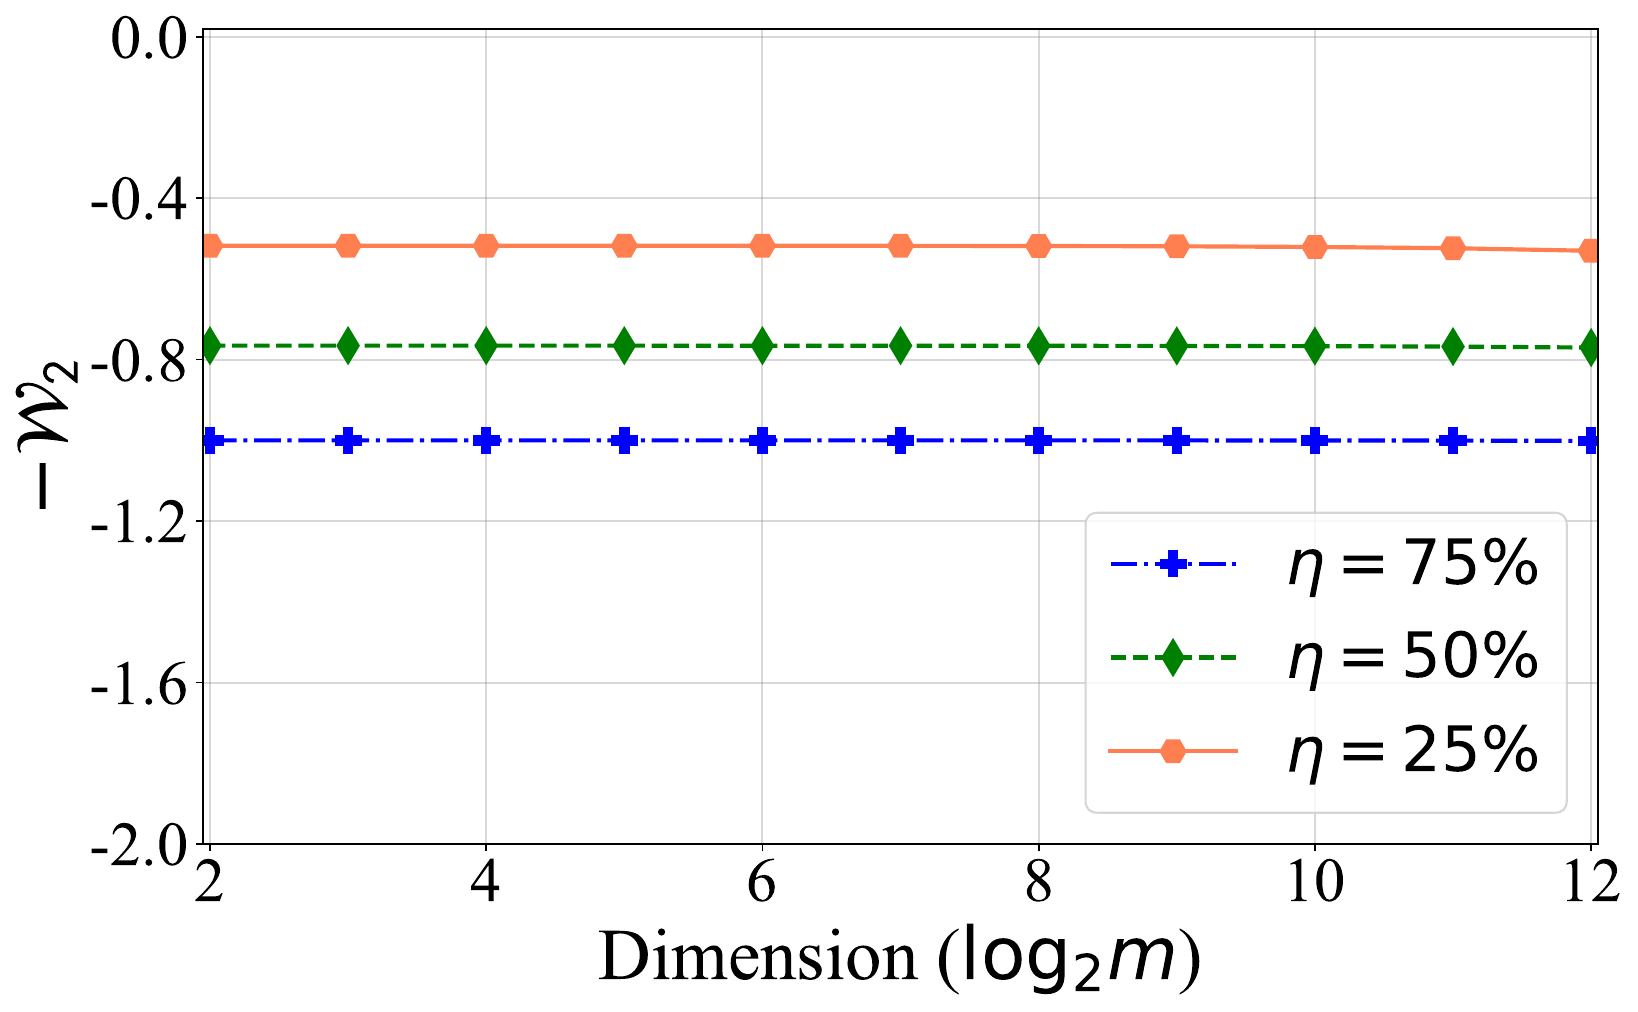}
	}
	\caption{\small{Dimensional collapse analysis w.r.t various dimensions. $\mathcal{L_U}$ fails to identify the dimensional collapse with a large dimension, while the ability of $\mathcal{W}_{2}$ to identify the dimensional collapse is free from the influence of dimensions.}}
	\vspace{-4mm}
	\label{fig:collapse analysis on dimension}
\end{figure*}
%%%%%%%%%%%%%%%%%%%%%%%%%%%%%%%%%%%%%%%%%%%%%%%%%%%%%%%%%%%%%%
\section{Parameter Setting in The Experiments}
\label{sec:parameter setting}
In Section~\ref{sec:experiment}, we impose the proposed uniformity metric, i.e., Wassserstein distance in Equation~\ref{eq:wasserstein distance} as an additional loss for various existing self-supervised methods. To adapt different models, we adopt a linear decay for weighting Wasserstein distance, and specific parameter setting is shown in Table~\ref{table:parameter setting}.
\begin{table*}[h]
\centering
\caption{Parameter setting for various models in experiments.}
\label{table:parameter setting}
\resizebox{0.60\textwidth}{!}{
\begin{tabular}{l c c c c} \hline
Models & MoCo v2 & BYOL & BarlowTwins & Zero-CL \\\hline
$\alpha_{max}$ & 1.0 & 0.2 & 30.0 & 30.0 \\
$\alpha_{min}$ & 1.0 & 0.2 & 0 & 30.0 \\\hline
\end{tabular}}
\end{table*}

%%%%%%%%%%%%%%%%%%%%%%%%%%%%%%%%%%%%%
\section{Alignment Metric for Self-Supervised Representation Learning}
\label{sec:alignment metric}
As one of the important indicators to evaluate representation capacity, the alignment metric measures the distance among semantically similar samples in the representation space, and smaller alignment generally brings better representation capacity. Wang et al~\citep{Wang2020UnderstandingCR} propose a simpler approach by calculating the average distance between the positive pairs as alignment, and it can be formulated as follows:
\begin{align}
\label{eq:alignment metric}
\mathcal{A} \triangleq \mathbb{E}_{(\m z^a_i, \m z^b_i)\sim p^{pos}_{\m z}} [\Vert \frac{\m z^a_i}{\Vert \m z^a_i \Vert} -\frac{\m z^b_i}{\Vert \m z^b_i \Vert}\Vert_2^{\beta}]
\end{align}
Where ($\m z^a_i$, $\m z^b_i$) is a positive pair as discussed in Section~\ref{sec:ssrl}. We set $\beta=2$ in the experiments.

\section{The Derivation of the pdf of $l_2$-normalized Gaussian distribution}
\begin{theorem}
For a random variable $\m Z \sim \mathcal{N}(\m 0, \sigma^2 \m I_m)$, and $\m Z \in \mathbb{R}^m$, for the $l_2$-normalized form $\m Y=\m Z/\Vert \m Z \Vert_2$, the probability density function(pdf) of a variable $Y_i$ in the arbitrary dimension is:
\label{proof:the pdf of y_i}
\begin{align}
\mathit{f}_{\scaleto{Y_i}{5pt}}(y_i) = \frac{\Gamma(m/2)}{\sqrt{\pi}\Gamma((m-1)/2)}(1-y_i^2)^{(m-3)/2} \nonumber
\end{align}
\end{theorem}
\begin{proof}
$\m Z=[Z_1, Z_2, \cdots, Z_m] \sim \mathcal{N}(\m 0, \sigma^2 \m I_m)$, then $Z_i \sim \mathcal{N}(0, \sigma^2) , \forall i \in [1, m]$. We denote the variable $U = Z_i/\sigma \sim \mathcal{N}(0, 1)$, $V = \sum_{j \neq i}^{m} (Z_j/\sigma)^2 \sim \mathcal{X}^2(m-1)$, then $U$ and $V$ are independent with each other. For the variable $T = \frac{U}{\sqrt{V/(m-1)}}$, it obeys the Student's t-distribution with $m-1$ degrees of freedom, and its probability density function (pdf) is:
\begin{align}
\nonumber \mathit{f}_{\scaleto{T}{5pt}}(t) = \frac{\Gamma(m/2)}{\sqrt{(m-1)\pi}\Gamma((m-1)/2)} (1+\frac{t^2}{m-1})^{-m/2}
\end{align}
For the variable $Y_i = \frac{Z_i}{\sqrt{\sum_{i=1}^{m}Z_i^2}} = \frac{Z_i}{\sqrt{Z_i^2 + \sum_{j \neq i}^{m} Z_j^2}} = \frac{Z_i/\sigma}{\sqrt{(Z_i/\sigma)^2 + \sum_{j \neq i}^{m} (Z_j/\sigma)^2}} = \frac{U}{\sqrt{U^2 + V}}$, then $T = \frac{U}{\sqrt{V/(m-1)}} = \frac{\sqrt{m-1}Y_i}{\sqrt{1-Y_i^2}}$ and $Y_i = \frac{T}{\sqrt{T^2+m-1}}$, the relation between the cumulative distribution function (cdf) of $T$ and that of $Y_i$ can be formulated as follows:
\begin{align}
\nonumber F_{Y_i}(y_i) = P(\{Y_i \leq y_i\}) &= 
\begin{cases}
P(\{Y_i \leq y_i\}) & y_i \leq 0 \\
P(\{Y_i \leq 0\}) +P(\{0 < Y_i \leq y_i\}) & y_i > 0
\end{cases} \\\nonumber
& = \begin{cases}
P(\{ \frac{T}{\sqrt{T^2+m-1}} \leq y_i\}) & y_i \leq 0 \\
P(\{ \frac{T}{\sqrt{T^2+m-1}} \leq 0\}) +P(\{0 < \frac{T}{\sqrt{T^2+m-1}} \leq y_i\}) & y_i > 0
\end{cases} \\\nonumber
& = \begin{cases}
P(\{ \frac{T^2}{T^2+m-1} \geq y_i^2, T \leq 0\}) & y_i \leq 0 \\
P(\{ T \leq 0\} +P(\{ \frac{T^2}{T^2+m-1} \leq y_i^2, T>0 \}) & y_i > 0
\end{cases} \\\nonumber
& = \begin{cases}
P(\{ T \leq \frac{\sqrt{m-1}y_i}{\sqrt{1-y_i^2}} \}) & y_i \leq 0 \\
P(\{ T \leq 0\} +P(\{ 0< T \leq \frac{\sqrt{m-1}y_i}{\sqrt{1-y_i^2}}\}) & y_i > 0
\end{cases} \\\nonumber
& = P(\{ T \leq \frac{\sqrt{m-1}y_i}{\sqrt{1-y_i^2}} \}) = F_{T}(\frac{\sqrt{m-1}y_i}{\sqrt{1-y_i^2}})
\end{align}
Therefore, the pdf of $Y_i$ can be derived as follows:
\begin{align}
\nonumber \mathit{f}_{\scaleto{Y_i}{5pt}}(y_i) & = \frac{d }{dy_i}F_{Y_i}(y_i) = \frac{d }{dy_i}F_{T}(\frac{\sqrt{m-1}y_i}{\sqrt{1-y_i^2}}) \\\nonumber
& = \mathit{f}_{\scaleto{T}{5pt}}(\frac{\sqrt{m-1}y_i}{\sqrt{1-y_i^2}}) \frac{d}{dy_i} (\frac{\sqrt{m-1}y_i}{\sqrt{1-y_i^2}}) \\\nonumber
& = [\frac{\Gamma(m/2)}{\sqrt{(m-1)\pi}\Gamma((m-1)/2)} (1-y_i^2)^{m/2}] [\sqrt{m-1} (1-y_i^2)^{-3/2}] \\\nonumber
& = \frac{\Gamma(m/2)}{\sqrt{\pi}\Gamma((m-1)/2)}(1-y_i^2)^{(m-3)/2}
\end{align}
\end{proof}

\section{The Kullback-Leibler Divergence between $Y_i$ and $\hat{Y}_i$}
\begin{theorem}
For a random variable $Y_i$ in the $i$-th dimension of $\m Y=\m Z/\Vert \m Z \Vert_2$,  where $\m Z \sim \mathcal{N}(\m 0, \sigma^2 \m I_m)$ ($\m Z \in \mathbb{R}^m$), then the Kullback-Leibler divergence between $Y_i$ and the variable $\hat{Y}_i \sim \mathcal{N}(0, \frac{1}{m})$ converges to zero as $m \to \infty$ as follows.
\label{proof:the kl divergence}
\begin{align}
\nonumber \lim\limits_{m \to \infty} \mathcal{D}_{KL}(\hat{Y}_i, Y_i) \to 0
\end{align}
\end{theorem}
\begin{proof}
For the variable $\hat{Y}_i \sim \mathcal{N}(0, \frac{1}{m})$, its pdf and $k$-th order raw moment can be formulated as:
\begin{align}
\nonumber \mathit{f}_{\scaleto{\hat{Y}_i}{5pt}}(y) = \sqrt{\frac{m}{2\pi}} \exp\{-\frac{my^2}{2}\}, \quad \mathbb{E}[\hat{Y}_i^k] =  \begin{cases}
\frac{\prod_{j=1}^{k/2} (2j-1) }{m^j} & k = 2j, j = 1,2,3... \\
0 & k = 2j-1
\end{cases}
\end{align}
According to the Theorem~\ref{proof:the pdf of y_i}, the pdf of $Y_i$ is:
\begin{align}
\mathit{f}_{\scaleto{Y_i}{5pt}}(y_i) = \frac{\Gamma(m/2)}{\sqrt{\pi}\Gamma((m-1)/2)}(1-y_i^2)^{(m-3)/2} \nonumber
\end{align}
For $0 \leq y <1$, the Taylor expansion of $\log (1-y^2)$ can be writted as:
\begin{align}
\nonumber \log (1-y^2) = -\sum_{j=1}^{\infty} \frac{y^{2j}}{j}
\end{align}
Then the Kullback-Leibler divergence between $\hat{Y}_i$ and $Y_i$ can be formulated as:
\begin{align}
\nonumber \mathcal{D}_{KL}(\hat{Y}_i, Y_i) & = \int_{-\infty}^{\infty} \mathit{f}_{\scaleto{\hat{Y}_i}{5pt}}(y) [\log \mathit{f}_{\scaleto{\hat{Y}_i}{5pt}}(y)- \log \mathit{f}_{\scaleto{Y_i}{5pt}}(y_i)] dy \\\nonumber
& = \int_{-\infty}^{\infty} \mathit{f}_{\scaleto{\hat{Y}_i}{5pt}}(y) [\log\sqrt{\frac{m}{2\pi}}-\frac{my^2}{2} - \log \frac{\Gamma(m/2)}{\sqrt{\pi}\Gamma((m-1)/2)} -\frac{m-3}{2} \log (1-y^2)] dy \\\nonumber
& = \log\sqrt{\frac{m}{2\pi}} - \log \frac{\Gamma(m/2)}{\sqrt{\pi}\Gamma((m-1)/2)} + \int_{-\infty}^{\infty} \mathit{f}_{\scaleto{\hat{Y}_i}{5pt}}(y) [-\frac{my^2}{2}-\frac{m-3}{2} \log (1-y^2)] \\\nonumber
& = \log \sqrt{\frac{m}{2}}\frac{\Gamma((m-1)/2)}{\Gamma(m/2)} + \int_{-\infty}^{\infty} \mathit{f}_{\scaleto{\hat{Y}_i}{5pt}}(y) [-\frac{my^2}{2} + \frac{m-3}{2} \sum_{j=1}^{\infty} \frac{y^{2j}}{j} ] \\\nonumber 
& = \log \sqrt{\frac{m}{2}}\frac{\Gamma((m-1)/2)}{\Gamma(m/2)} - \frac{m}{2}\mathbb{E}(\hat{Y}_i^{2}) + \frac{m-3}{2} \sum_{j=1}^{\infty} \mathbb{E}(\hat{Y}_i^{2j})/j\\\nonumber
& = \log \sqrt{\frac{m}{2}}\frac{\Gamma((m-1)/2)}{\Gamma(m/2)} -\frac{1}{2} + \frac{m-3}{2} [\frac{1}{m} + \frac{3}{2m^2} + \frac{5*3}{3m^3} + o(\frac{1}{m^3})]
\end{align}
According to the Stirling formula, we $\Gamma(x+\alpha) \sim \Gamma(x)x^{\alpha}$ as $x \to \infty $, therefore:
\begin{align}
\nonumber \lim\limits_{m \to \infty} \log \sqrt{\frac{m}{2}}\frac{\Gamma((m-1)/2)}{\Gamma(m/2)} & = \lim\limits_{m \to \infty} \log \sqrt{\frac{m}{2}} \frac{\Gamma((m-1)/2)}{\Gamma((m-1)/2)(\frac{m-1}{2})^{1/2}} \\\nonumber
& = \lim\limits_{m \to \infty} \log \sqrt{\frac{m}{2}} \sqrt{\frac{2}{m-1}} = 0
\end{align}
Then the Kullback-Leibler divergence between $\hat{Y}_i$ and $Y_i$ converges to zero as $m \to \infty$ as follows:
\begin{align}
\nonumber \lim\limits_{m \to \infty} \mathcal{D}_{KL}(\hat{Y}_i, Y_i) &= \lim\limits_{m \to \infty} \log \sqrt{\frac{m}{2}}\frac{\Gamma((m-1)/2)}{\Gamma(m/2)} -\frac{1}{2} + \frac{m-3}{2} [\frac{1}{m} + \frac{3}{2m^2} + \frac{5*3}{3m^3} + o(\frac{1}{m^3})] \\\nonumber 
& = 0 + \lim\limits_{m \to \infty} -\frac{1}{2} + \frac{m-3}{2} [\frac{1}{m} + \frac{3}{2m^2} + \frac{5*3}{3m^3} + o(\frac{1}{m^3})] = 0
\end{align}
\end{proof}
